# Supplementary material for: Exact percolation probabilities for a square lattice: Site percolation on a plane, cylinder, and torus
Source: arXiv:2204.01517 ancillary file (2022-03-31)
Supplement: Supplementary file 1 [file Algorithm2.pdf]

## Algorithm 2 for a cylinder or a torus

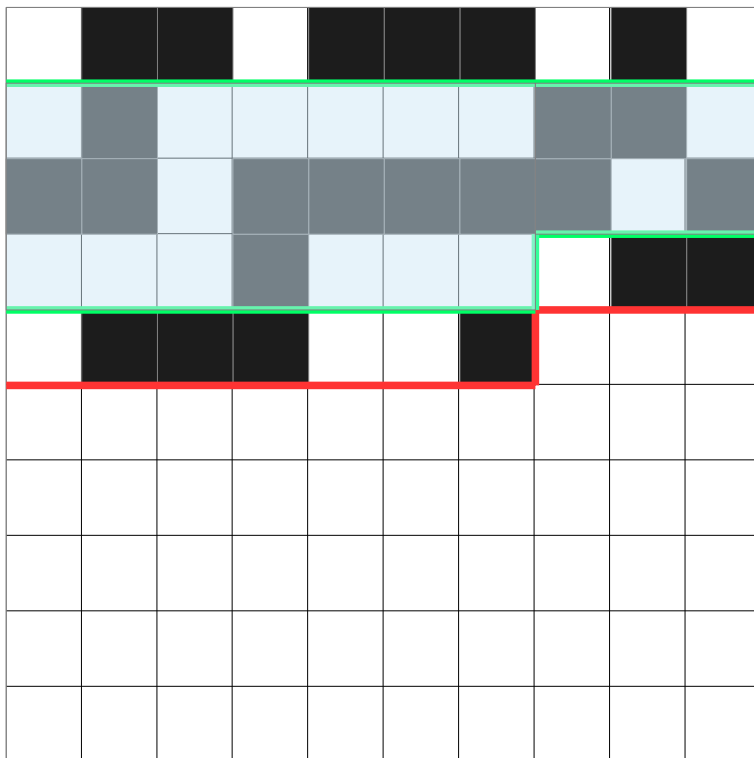

Figure 1. Situation S.

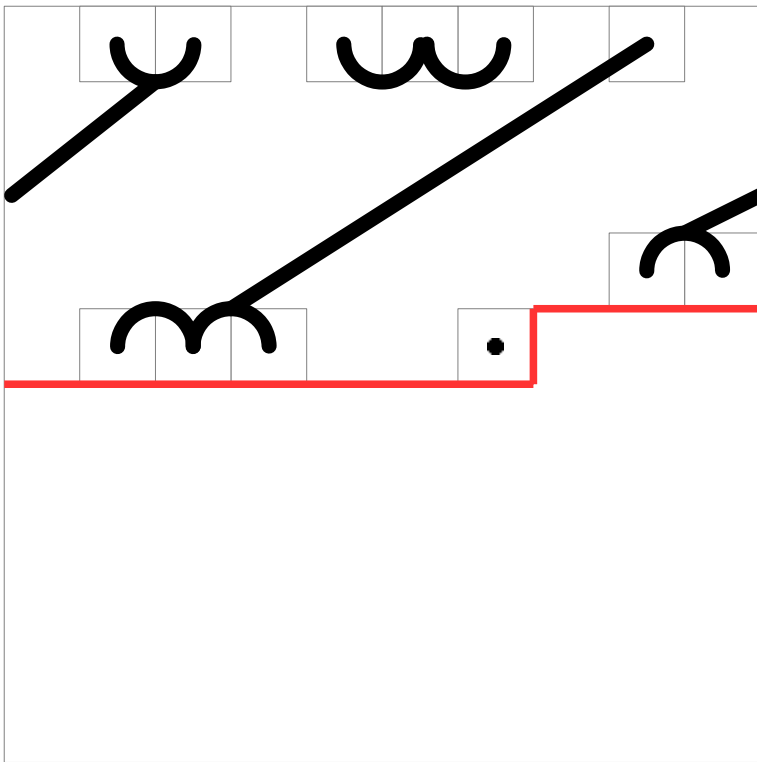

Figure 2. Topological representation of situation S.

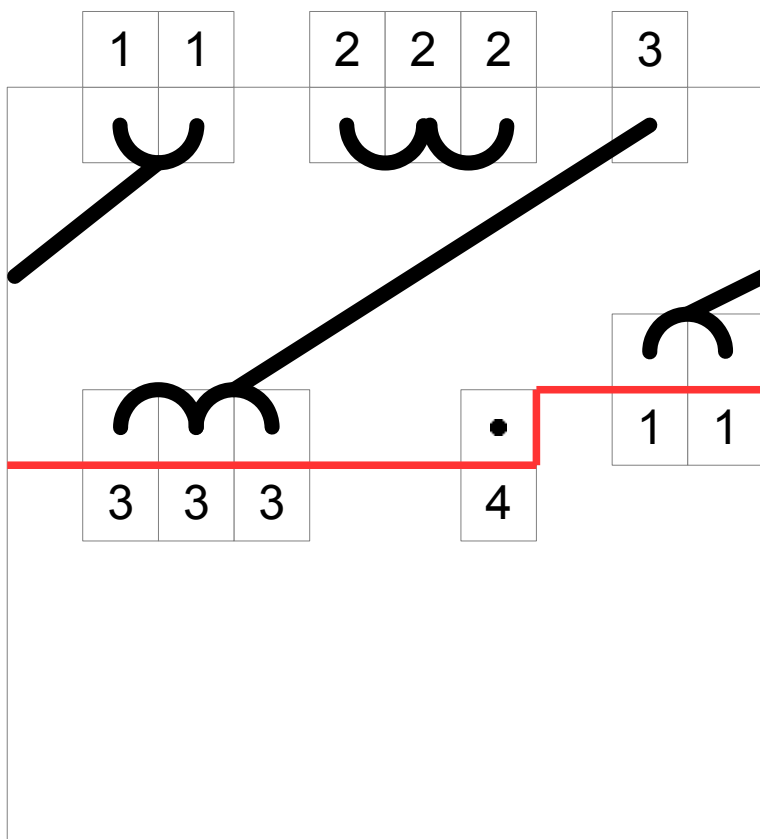

|   |   |   |   |   |   |   |   |   |   |
|---|---|---|---|---|---|---|---|---|---|
| 0 | 1 | 1 | 0 | 2 | 2 | 2 | 0 | 3 | 0 |
|---|---|---|---|---|---|---|---|---|---|

|   |   |   |   |   |   |   |   |   |   |
|---|---|---|---|---|---|---|---|---|---|
| 0 | 3 | 3 | 3 | 0 | 0 | 4 | 0 | 1 | 1 |
|---|---|---|---|---|---|---|---|---|---|

Figure 3. Signature of the situation S.

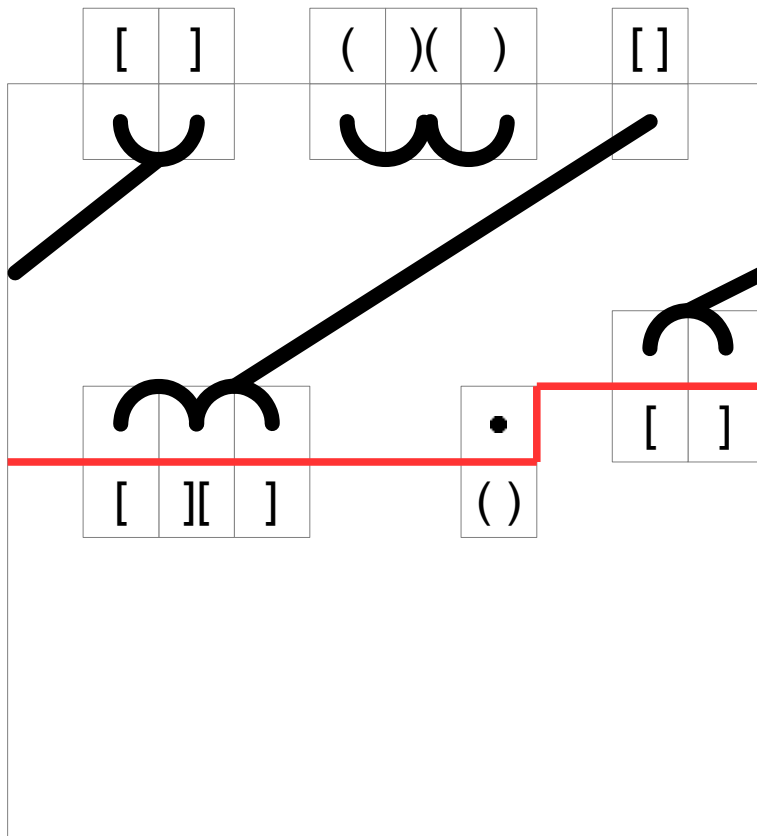

|  |   |   |  |   |   |  |   |   |
|--|---|---|--|---|---|--|---|---|
|  | [ | ] |  | ( | ) |  | [ | ] |
|--|---|---|--|---|---|--|---|---|

|  |   |   |   |   |  |  |   |   |  |   |   |
|--|---|---|---|---|--|--|---|---|--|---|---|
|  | [ | ] | [ | ] |  |  | ( | ) |  | [ | ] |
|--|---|---|---|---|--|--|---|---|--|---|---|

Figure 4. Bracket notation of the situation S (the notation is equivalent to the notation in S.Mertens) without taking into account the matching of spanning clusters.



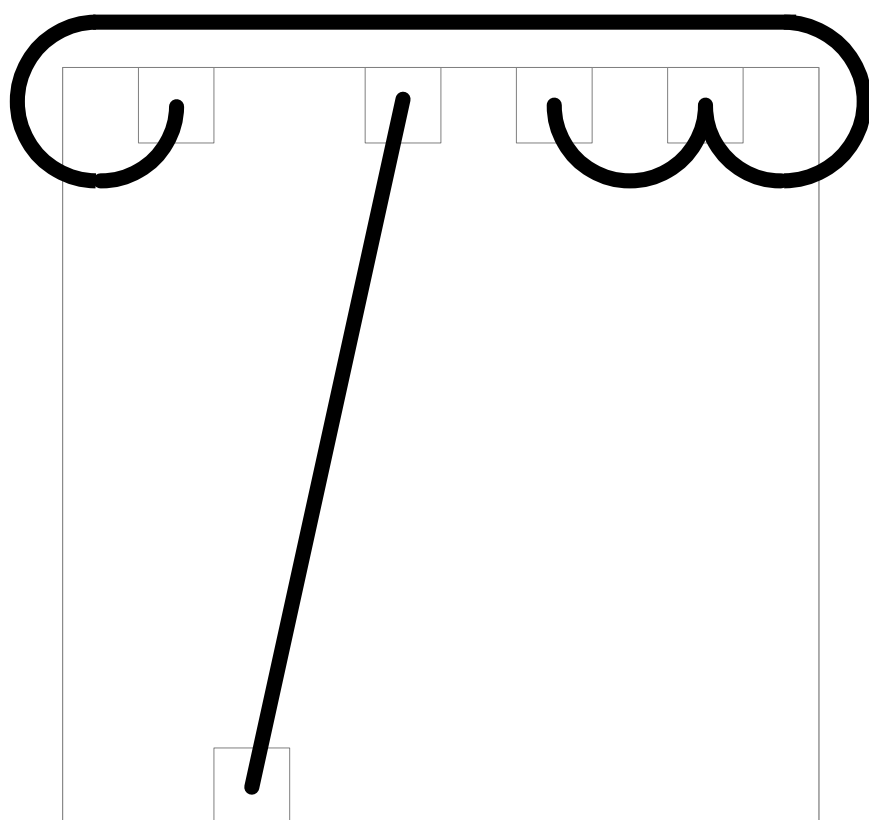

|  |   |  |  |   |  |   |  |   |  |
|--|---|--|--|---|--|---|--|---|--|
|  | 1 |  |  | 2 |  | 1 |  | 1 |  |
|--|---|--|--|---|--|---|--|---|--|

|  |  |   |  |  |  |  |  |  |  |
|--|--|---|--|--|--|--|--|--|--|
|  |  | 2 |  |  |  |  |  |  |  |
|--|--|---|--|--|--|--|--|--|--|

Figure 6. Topological representation of situation S and its signature.

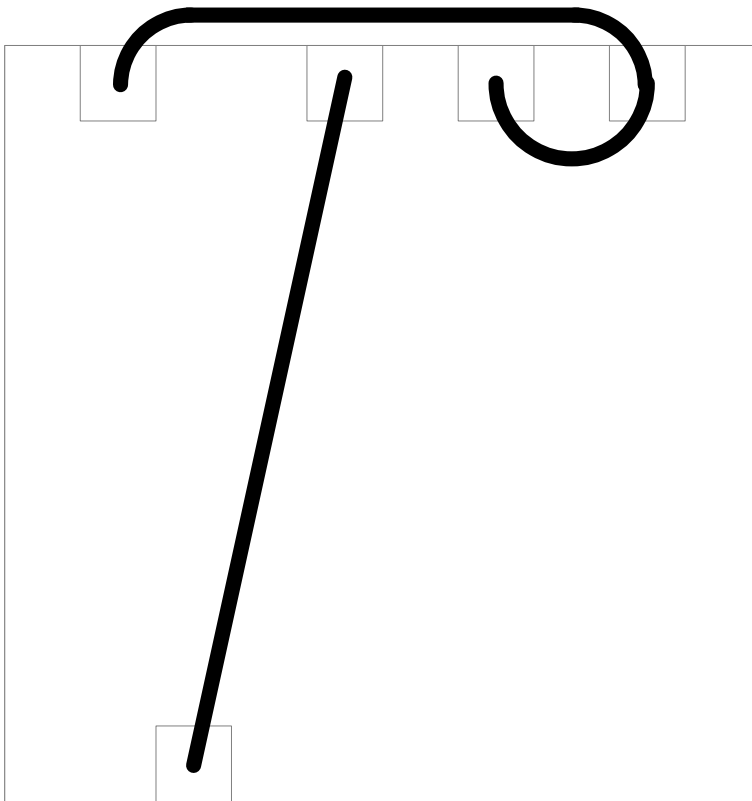

|  |   |  |  |   |  |   |  |   |  |
|--|---|--|--|---|--|---|--|---|--|
|  | 1 |  |  | 2 |  | 1 |  | 1 |  |
|--|---|--|--|---|--|---|--|---|--|

|  |  |   |  |  |  |  |  |  |  |
|--|--|---|--|--|--|--|--|--|--|
|  |  | 2 |  |  |  |  |  |  |  |
|--|--|---|--|--|--|--|--|--|--|

Figure 7. Modification of the topological representation of the situation S.

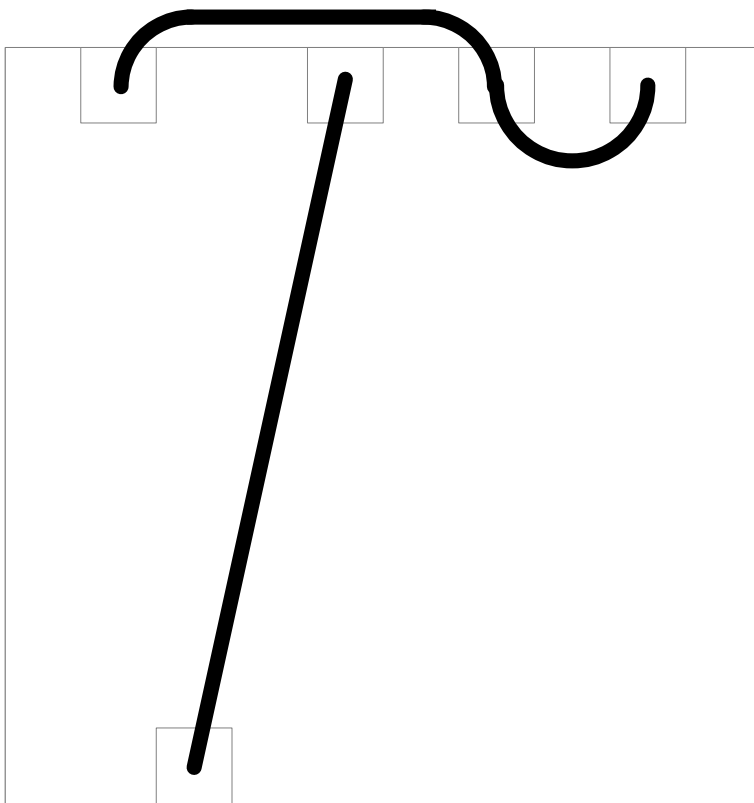

|  |   |  |  |   |  |   |   |  |   |  |
|--|---|--|--|---|--|---|---|--|---|--|
|  | ( |  |  | * |  | ) | ( |  | ) |  |
|--|---|--|--|---|--|---|---|--|---|--|

|  |  |   |  |  |  |  |  |  |  |
|--|--|---|--|--|--|--|--|--|--|
|  |  | * |  |  |  |  |  |  |  |
|--|--|---|--|--|--|--|--|--|--|

Figure 8. The final modification of the topological representation of the situation S and its bracket notation with a label specifying the matching of spanning clusters.
